# Supplementary material for: Concavity Effects on the Optical Properties of Aromatic Hydrocarbons
Source: arXiv:1306.2766 source file (2013-06-12)
Supplement: Supplementary file 1 [file supp_info.pdf]

# SUPPORTING INFORMATION

# Concavity Effects on the Optical Properties of Aromatic Hydrocarbons

Caterina Cocchi,*,† Deborah Prezzi,† Alice Ruini,†,‡ Marilia J. Caldas,¶ Annalisa Fasolino,§ and Elisa Molinari†,‡

*Centro S3, CNR-Istituto Nanoscienze, I-41125 Modena, Italy, Dipartimento di Scienze Fisiche, Informatiche e Matematiche, Università di Modena e Reggio Emilia, I-41125 Modena, Italy, Instituto de Física, Universidade de São Paulo, 05508-900 São Paulo, SP, Brazil, and Institute for Molecules and Materials, Radboud University Nijmegen, Heyendaalseweg 135, 6525AJ Nijmegen, The Netherlands*

E-mail: caterina.cocchi@unimore.it

*To whom correspondence should be addressed

†Centro S3, CNR-Istituto Nanoscienze, I-41125 Modena, Italy

‡Dipartimento di Scienze Fisiche, Informatiche e Matematiche, Università di Modena e Reggio Emilia, I-41125 Modena, Italy

¶Instituto de Física, Universidade de São Paulo, 05508-900 São Paulo, SP, Brazil

§Institute for Molecules and Materials, Radboud University Nijmegen, Heyendaalseweg 135, 6525AJ Nijmegen, The Netherlands

# Electronic Properties of Concave PAHs

We report the ionization potential (IP) and the electron affinity (EA) computed for the series of concave polycyclic aromatic hydrocarbons (PAHs) $C_{60}H_{6n}$ ($n$ = 0, ..., 5) (Table S1) and $C_{50}H_{10m}$ ($m$ = 1,2) (Table S2). These values are calculated by means of the semi-empirical model AM1, as the difference between the total energy of neutral and (±1) charged states: EA = E(0) - E(-1) and IP = E(+1) - E(0).

**Table S1: Electron affinity (EA) and ionization potential (IP) of the series of PAHs $C_{60}H_{6n}$ ($n$ = 0, ..., 5). These values are computed with AM1 as the difference between the total energy of neutral and (±1) charged states: EA = E(0) - E(-1) and IP = E(+1) - E(0).**

| Structure | $C_{60}H_{30}$ | $C_{60}H_{24}$ | $C_{60}H_{18}$ | $C_{60}H_{12}$ | $C_{60}H_{6}$ | $C_{60}$ |
|---|---|---|---|---|---|---|
| EA (eV) | 1.66 | 2.03 | 2.00 | 2.41 | 2.82 | 3.07 |
| IP (eV) | 7.67 | 8.23 | 8.37 | 8.76 | 8.96 | 9.46 |

The values of EA and IP computed for $C_{60}$ (see Table S1) are consistent with previous results, obtained with MNDO model.[1,2]

**Table S2: Electron affinity (EA) and ionization potential (IP) of pentaindenocorannulene $C_{50}H_{20}$ and the carbon-nanotube-cap $C_{50}H_{10}$. These values are computed with AM1 as the difference between the total energy of neutral and (±1) charged states, i.e. EA = E(0) - E(-1) and IP = E(+1) - E(0).**

| Structure | $C_{50}H_{20}$ | $C_{50}H_{10}$ |
|---|---|---|
| EA (eV) | 1.95 | 2.35 |
| IP (eV) | 8.25 | 8.51 |

By inspecting Table S1 and Table S2, we notice that both EA and IP increase along with the dehydrogenation and the increasing $\pi$-connectivity of both series of PAHs. These quantities can hence be seen as indicators of structural stabilization of the molecules, from the initial planar precursor, up to the closed fullerene cage.

# Optical Excitations of $C_{60}$

In this section we extend the discussion on the first excitations of $C_{60}$, by reporting our results and comparing them with theoretical (at ZINDO/S level) and experimental data, available in the literature.

**Table S3: Lowest energy optical excitations of $C_{60}$ with icosahedral symmetry ($I_h$ point group). In addition to the energies and the oscillator strength (OS), also the symmetry is indicated, together with the degeneracy (deg) of the excitation.**

| Symmetry (deg) | Energy (eV) | OS |
|---|---|---|
| $^1T_{1g}$ (3) | 2.38 | $< 10^{-6}$ |
| $^1T_{2g}$ (3) | 2.39 | $< 10^{-6}$ |
| $^1G_g$ (4) | 2.40 | $< 10^{-6}$ |
| $^1H_g$ (5) | 2.71 | $< 10^{-6}$ |
| $^1T_{2u}$ (3) | 2.81 | $< 10^{-6}$ |
| $^1H_u$ (5) | 3.08 | $< 10^{-6}$ |
| $^1G_u$ (4) | 3.21 | $< 10^{-6}$ |
| $^1T_{1u}$ (3) | 3.30 | $0.7 \times 10^{-4}$ |
| $^1T_{1u}$ (3) | 4.07 | 0.56 |

The first seven excited states of $C_{60}$, shown in Table S3, are dipole forbidden. All these excitations present multiple degeneracy, due to the high symmetry of $C_{60}$ ($I_h$ point group). Manifolds of three-, four- and five-fold degenerate states are obtained: these features are also evident in the optical spectrum of fullerene shown in Figure 2. Our results are consistent with the findings of Bendale and coworkers,[3] although our excitation energies are systematically higher of about 120-150 meV. This feature can be ascribed to the different CI windows adopted: in Ref.[3] 30 occupied and 35 empty states are considered, while we included 38 occupied and 37 empty orbitals. Moreover Bendale and coworkers performed geometry optimization using a INDO/1 Hamiltonian.[3] Their C-C bond lengths present differences of the order of 0.01 Å with respect to those computed by AM1 in our work.

It is worth pointing out the good agreement between our results and the experimental data presented in the same paper,[3] although in experiments the excited states between about 2.5 and 3 eV are not dark, but give rise to weak signals. This behavior is explained by the presence

of the solvent and by the spontaneous symmetry breaking of the molecule in typical laboratory conditions. In Table S3 we also include the first visible excitations of $C_{60}$, of symmetry $T_{1u}$ and hence dipole allowed, which are labelled as $B_w$ and $B_m$ in the text, borrowing the notation of Bendale and coworkers, according to the peak intensity (*w* stands for *weak* and *m* for *medium*). Both these bright states are three-fold degenerate.

## Optical Excitations of Pentaindenocorannulene ($C_{50}H_{20}$) and Carbon-Nanotube-Cap ($C_{50}H_{10}$)

In Table S4 we report the energy and oscillator strength (OS) of the main excitations $D_1$, $B_{xy}$ and $B_z$, identified in the optical spectra of $C_{50}H_{20}$ and $C_{50}H_{10}$ (see main text, Figure 4).

**Table S4: Energy and oscillator strength (OS) of the main excitations of pentaindenocorannulene ($C_{50}H_{20}$) and carbon-nanotube-cap ($C_{50}H_{10}$). The single (s) or double (d) degeneracy is indicated for each excitation.**

| Structure | $D_1$ | | $B_{xy}$ | | $B_z$ | |
|---|---|---|---|---|---|---|
| | **Energy (eV)** | **OS** | **Energy (eV)** | **OS** | **Energy (eV)** | **OS** |
| $C_{50}H_{20}$ | 2.90 (s) | 0.00 | 3.11 (d) | 0.12 | 5.18 (s) | 0.10 |
| $C_{50}H_{10}$ | 2.28 (s) | 0.00 | 3.50 (d) | 0.09 | 5.00 (s) | 1.24 |

The first dark state is singly degenerate, in agreement also with the behavior of the $C_{60}H_{6n}$ series. The bright peaks $B_{xy}$ and $B_z$ present double and single degeneracy, respectively: while the former is polarized in the $(x, y)$-plane and hence is symmetric in these directions, according to the properties of $C_{5v}$ point group symmetry, the latter is polarized in the out-of-plane direction ($z$). As such, its OS increases of one order of magnitude from $C_{50}H_{20}$ to $C_{50}H_{10}$ (see also Figure 4 in the main text).

## Optical Excitations of Zipped PAHs

In Table S5 we report the energy and OS of the main excitations $D_1$, $B_L$ and $B_T$, identified in the optical spectra of planar ($C_{60}H_{22}$), etched ($C_{58}H_{20}$) and zipped ($C_{58}H_{16}$) PAHs (see main text,

**Table S5: Energy and oscillator strength (OS) of the main excitations of planar ($C_{60}H_{22}$), etched ($C_{58}H_{20}$) and zipped ($C_{58}H_{16}$) PAHs.**

| Structure | $D_1$ | | $B_L$ | | $B_T$ | |
|---|---|---|---|---|---|---|
| | **Energy (eV)** | **OS** | **Energy (eV)** | **OS** | **Energy (eV)** | **OS** |
| $C_{60}H_{22}$ | - | - | 1.54 | 1.63 | 2.58 | 1.27 |
| $C_{58}H_{20}$ | - | - | 1.98 | 0.57 | 2.98 | 0.98 |
| $C_{58}H_{16}$ | 1.16 | 0.00 | 2.34 | 0.11 | 2.69 | 0.40 |

Figure 5).

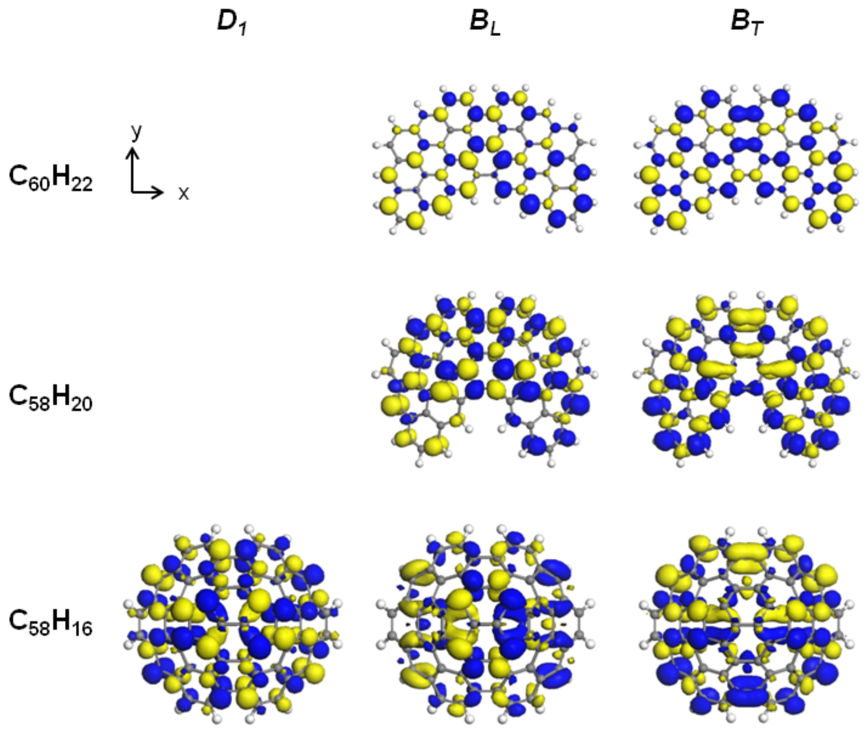


Figure S1: Top view $(x,y)$ of the transition density plots of the excitations of zipped PAHs $C_{60}H_{22}$, $C_{58}H_{20}$ and $C_{58}H_{16}$. The first dark excited state $D_1$ is observed only in the zipped concave molecule $C_{58}H_{16}$. The bright excitations are labelled in this series as $B_L$ and $B_T$, according to their polarization along the longitudinal ($x$) or transverse ($y$) direction of the molecules.

According to their structure and shape, the PAHs of this series are characterized by singly degenerate bright peaks polarized along the longitudinal ($x$) and transverse ($y$) axes of the molecules (see Figure S1). Their are labelled following this notation, both in Table S5 here and in Figure 5b in the main text. The longitudinal and transverse polarization character of these bright excitations is evidently represented in the plots of their transition densities (TD) shown in Figure S1. It is

worth noting that the first dark excitation $D_1$ is present only in the spectrum of the zipped concave molecule $C_{58}H_{16}$. The sign modulation of its TD (see Figure S1) clearly account for its vanishing intensity.

## References


(1) Newton, M. D.; Stanton, R. E. *J. Am. Chem. Soc.* **1986**, *108*, 2469–2470.

(2) Bakowies, D.; Thiel, W. *J. Am. Chem. Soc.* **1991**, *113*, 3704–3714.

(3) Bendale, R.; Baker, J.; Zerner, M. *Int. J. Quantum Chem.* **1991**, *40*, 557–568.
